# Supplementary material for: A Hetero-functional Graph State Estimator for Watershed Systems: Application to the Chesapeake Bay
Source: arXiv:2603.01931 source file (2026-11-03)
Supplement: Supplementary file 1 [file supplement.tex]

\relax 
\providecommand \babel@aux [2]{\global \let \babel@toc \@gobbletwo }
\@nameuse{bbl@beforestart}
\providecommand\hyper@newdestlabel[2]{}
\providecommand\HyField@AuxAddToFields[1]{}
\providecommand\HyField@AuxAddToCoFields[2]{}
\bibstyle{opticajnl}
\citation{weck:2011:00}
\citation{Walden:2015:00}
\citation{Hoyle:1998:00,Walden:2015:00}
\citation{Walden:2015:00}
\citation{Walden:2015:00,Hoyle:1998:00}
\babel@aux{english}{}
\@writefile{toc}{\contentsline {section}{\numberline {S1}Hetero-functional Graph Theory Meta\hyp  {}Architecture \& Definitions}{1}{section.1}\protected@file@percent }
\newlabel{sec:cbw-hfgt}{{S1}{1}{Hetero-functional Graph Theory Meta\hyp {}Architecture \& Definitions}{section.1}{}}
\@writefile{loe}{\contentsline {defn}{\ifthmt@listswap Definition~S1\else \numberline {S1}Definition\fi \thmtformatoptarg {Engineering System \cite  {weck:2011:00}}}{1}{defn.1}\protected@file@percent }
\newlabel{defn:cbw-EngineeringSystem}{{S1}{1}{Engineering System \cite {weck:2011:00}}{defn.1}{}}
\@writefile{loe}{\contentsline {defn}{\ifthmt@listswap Definition~S2\else \numberline {S2}Definition\fi \thmtformatoptarg {System Operand \cite  {Walden:2015:00}}}{1}{defn.2}\protected@file@percent }
\newlabel{def:cbw-operand}{{S2}{1}{System Operand \cite {Walden:2015:00}}{defn.2}{}}
\@writefile{loe}{\contentsline {defn}{\ifthmt@listswap Definition~S3\else \numberline {S3}Definition\fi \thmtformatoptarg {System Process \cite  {Hoyle:1998:00,Walden:2015:00}}}{1}{defn.3}\protected@file@percent }
\newlabel{def:cbw-process}{{S3}{1}{System Process \cite {Hoyle:1998:00,Walden:2015:00}}{defn.3}{}}
\@writefile{loe}{\contentsline {defn}{\ifthmt@listswap Definition~S4\else \numberline {S4}Definition\fi \thmtformatoptarg {System Resource \cite  {Walden:2015:00}}}{1}{defn.4}\protected@file@percent }
\newlabel{def:cbw-resource}{{S4}{1}{System Resource \cite {Walden:2015:00}}{defn.4}{}}
\citation{Schoonenberg:2019:00,Farid:2022:00}
\citation{Schoonenberg:2019:00,Farid:2022:00}
\citation{Schoonenberg:2019:00,Farid:2022:00,Farid:2016:ISC-BC06}
\citation{Schoonenberg:2019:00}
\citation{Schoonenberg:2019:00}
\citation{Farid:2022:00}
\citation{Farid:2022:00}
\@writefile{loe}{\contentsline {defn}{\ifthmt@listswap Definition~S5\else \numberline {S5}Definition\fi \thmtformatoptarg {Buffer \cite  {Schoonenberg:2019:00,Farid:2022:00}}}{2}{defn.5}\protected@file@percent }
\newlabel{def:cbw-buffer}{{S5}{2}{Buffer \cite {Schoonenberg:2019:00,Farid:2022:00}}{defn.5}{}}
\@writefile{loe}{\contentsline {defn}{\ifthmt@listswap Definition~S6\else \numberline {S6}Definition\fi \thmtformatoptarg {Capability \cite  {Schoonenberg:2019:00,Farid:2022:00,Farid:2016:ISC-BC06}}}{2}{defn.6}\protected@file@percent }
\newlabel{def:cbw-capability}{{S6}{2}{Capability \cite {Schoonenberg:2019:00,Farid:2022:00,Farid:2016:ISC-BC06}}{defn.6}{}}
\@writefile{loe}{\contentsline {defn}{\ifthmt@listswap Definition~S7\else \numberline {S7}Definition\fi \thmtformatoptarg {The Negative 3$^{rd}$ Order Hetero-functional Incidence Tensor (HFIT) $\setbox \z@ \hbox {\mathsurround \z@ $\textstyle \cal  M$}\mathaccent "0365{\cal  M}_\rho ^-$\cite  {Farid:2022:00}}}{2}{defn.7}\protected@file@percent }
\newlabel{defn:cbw-D6}{{S7}{2}{The Negative 3$^{rd}$ Order Hetero-functional Incidence Tensor (HFIT) $\widetilde {\cal M}_\rho ^-$\cite {Farid:2022:00}}{defn.7}{}}
\@writefile{loe}{\contentsline {defn}{\ifthmt@listswap Definition~S8\else \numberline {S8}Definition\fi \thmtformatoptarg {The Positive 3$^{rd}$ Order Hetero-functional Incidence Tensor (HFIT)$\setbox \z@ \hbox {\mathsurround \z@ $\textstyle \cal  M$}\mathaccent "0365{\cal  M}_\rho ^+$\cite  {Farid:2022:00}}}{2}{defn.8}\protected@file@percent }
\@writefile{lof}{\contentsline {figure}{\numberline {S1}{\ignorespaces A SysML Block Definition Diagram of the System Form of the Engineering System Meta-Architecture. Adapted from {\cite  {Schoonenberg:2019:00}}.}}{3}{figure.caption.1}\protected@file@percent }
\providecommand*\caption@xref[2]{\@setref\relax\@undefined{#1}}
\newlabel{fig:cbw-LFESMetaArchitecturebdd}{{S1}{3}{A SysML Block Definition Diagram of the System Form of the Engineering System Meta-Architecture. Adapted from \protect {\cite {Schoonenberg:2019:00}}}{figure.caption.1}{}}
\@writefile{lof}{\contentsline {figure}{\numberline {S2}{\ignorespaces A SysML Activity Diagram of the System Function of the Engineering System Meta-Architecture. Adapted from {\cite  {Schoonenberg:2019:00}}.}}{3}{figure.caption.2}\protected@file@percent }
\newlabel{fig:cbw-LFESMetaArchitectureact}{{S2}{3}{A SysML Activity Diagram of the System Function of the Engineering System Meta-Architecture. Adapted from \protect {\cite {Schoonenberg:2019:00}}}{figure.caption.2}{}}
\citation{Schoonenberg:2022:ISC-J48}
\citation{Schoonenberg:2022:ISC-J48}
\citation{Schoonenberg:2022:ISC-J48}
\citation{Schoonenberg:2022:ISC-J48}
\citation{Farid:2008:IEM-J04,Schoonenberg:2019:00,Khayal:2018:00,Schoonenberg:2017:01}
\@writefile{loe}{\contentsline {defn}{\ifthmt@listswap Definition~S9\else \numberline {S9}Definition\fi \thmtformatoptarg {Engineering System Net \cite  {Schoonenberg:2022:ISC-J48}}}{4}{defn.9}\protected@file@percent }
\newlabel{defn:cbw-ESN}{{S9}{4}{Engineering System Net \cite {Schoonenberg:2022:ISC-J48}}{defn.9}{}}
\@writefile{loe}{\contentsline {defn}{\ifthmt@listswap Definition~S10\else \numberline {S10}Definition\fi \thmtformatoptarg {Engineering System Net State Transition Function \cite  {Schoonenberg:2022:ISC-J48}}}{4}{defn.10}\protected@file@percent }
\newlabel{defn:cbw-ESN-STF}{{S10}{4}{Engineering System Net State Transition Function \cite {Schoonenberg:2022:ISC-J48}}{defn.10}{}}
\newlabel{eq:cbw-PhiCPN}{{S1}{4}{Engineering System Net State Transition Function \cite {Schoonenberg:2022:ISC-J48}}{equation.1}{}}
\newlabel{eq:cbw-Q_B:HFNMCFprogram}{{S2}{4}{Engineering System Net State Transition Function \cite {Schoonenberg:2022:ISC-J48}}{equation.2}{}}
\newlabel{eq:cbw-Q_E:HFNMCFprogram}{{S3}{4}{Engineering System Net State Transition Function \cite {Schoonenberg:2022:ISC-J48}}{equation.3}{}}
\@writefile{loe}{\contentsline {defn}{\ifthmt@listswap Definition~S11\else \numberline {S11}Definition\fi \thmtformatoptarg {Operand Net~\cite  {Farid:2008:IEM-J04,Schoonenberg:2019:00,Khayal:2018:00,Schoonenberg:2017:01}}}{4}{defn.11}\protected@file@percent }
\newlabel{defn:cbw-OperandNet}{{S11}{4}{Operand Net~\cite {Farid:2008:IEM-J04,Schoonenberg:2019:00,Khayal:2018:00,Schoonenberg:2017:01}}{defn.11}{}}
\citation{Farid:2008:IEM-J04,Schoonenberg:2019:00,Khayal:2018:00,Schoonenberg:2017:01}
\citation{Schoonenberg:2017:01,Farid:2008:IEM-J04,Farid:2008:IEM-J05}
\citation{Khayal:2021:00,Khayal:2018:00,Khayal:2015:ISC-J20}
\citation{White:1994:00}
\citation{Farid:2025:ISC-BKR01}
\citation{Schoonenberg:2022:ISC-J48}
\citation{Thompson:2025:ISC-JR11}
\citation{Thompson:2025:ISC-JR11}
\citation{Thompson:2025:ISC-JR11}
\@writefile{loe}{\contentsline {defn}{\ifthmt@listswap Definition~S12\else \numberline {S12}Definition\fi \thmtformatoptarg {Operand Net State Transition Function~\cite  {Farid:2008:IEM-J04,Schoonenberg:2019:00,Khayal:2018:00,Schoonenberg:2017:01}}}{5}{defn.12}\protected@file@percent }
\newlabel{defn:cbw-OperandNet-STF}{{S12}{5}{Operand Net State Transition Function~\cite {Farid:2008:IEM-J04,Schoonenberg:2019:00,Khayal:2018:00,Schoonenberg:2017:01}}{defn.12}{}}
\newlabel{eq:cbw-PhiSPN}{{S4}{5}{Operand Net State Transition Function~\cite {Farid:2008:IEM-J04,Schoonenberg:2019:00,Khayal:2018:00,Schoonenberg:2017:01}}{equation.4}{}}
\newlabel{X}{{S5}{5}{Operand Net State Transition Function~\cite {Farid:2008:IEM-J04,Schoonenberg:2019:00,Khayal:2018:00,Schoonenberg:2017:01}}{equation.5}{}}
\newlabel{CH eq:Q_E:HFNMCFprogram}{{S6}{5}{Operand Net State Transition Function~\cite {Farid:2008:IEM-J04,Schoonenberg:2019:00,Khayal:2018:00,Schoonenberg:2017:01}}{equation.6}{}}
\@writefile{toc}{\contentsline {section}{\numberline {S2}Weighted Least Squares Error Hetero-functional Graph State Estimation}{5}{section.2}\protected@file@percent }
\newlabel{sec:cbw-WLSEHFGSE}{{S2}{5}{Weighted Least Squares Error Hetero-functional Graph State Estimation}{section.2}{}}
\newlabel{eq:cbw-WLSEHFGSE}{{S7}{6}{Weighted Least Squares Error Hetero-functional Graph State Estimation}{equation.7}{}}
\newlabel{eq:cbw-WLSEHFGSEOF}{{S7a}{6}{Weighted Least Squares Error Hetero-functional Graph State Estimation}{equation.7a}{}}
\newlabel{eq:cbw-EqualityConstraintsOC}{{S7b}{6}{Weighted Least Squares Error Hetero-functional Graph State Estimation}{equation.7b}{}}
\newlabel{eq:cbw-TransitionConstraint2}{{S7c}{6}{Weighted Least Squares Error Hetero-functional Graph State Estimation}{equation.7c}{}}
\newlabel{eq:cbw-DurationConstraint2}{{S7d}{6}{Weighted Least Squares Error Hetero-functional Graph State Estimation}{equation.7d}{}}
\newlabel{eq:cbw-SSN-STF-QB2}{{S7e}{6}{Weighted Least Squares Error Hetero-functional Graph State Estimation}{equation.7e}{}}
\newlabel{eq:cbw-OperandNet-STF2OC}{{S7f}{6}{Weighted Least Squares Error Hetero-functional Graph State Estimation}{equation.7f}{}}
\newlabel{eq:cbw-OperandNetDurationConstraint2}{{S7g}{6}{Weighted Least Squares Error Hetero-functional Graph State Estimation}{equation.7g}{}}
\newlabel{eq:cbw-SyncPlusOC}{{S7h}{6}{Weighted Least Squares Error Hetero-functional Graph State Estimation}{equation.7h}{}}
\newlabel{eq:cbw-SyncMinusOC}{{S7i}{6}{Weighted Least Squares Error Hetero-functional Graph State Estimation}{equation.7i}{}}
\newlabel{eq:cbw-ESNMeasurement}{{S7j}{6}{Weighted Least Squares Error Hetero-functional Graph State Estimation}{equation.7j}{}}
\newlabel{eq:cbw-SSNMeasurement}{{S7k}{6}{Weighted Least Squares Error Hetero-functional Graph State Estimation}{equation.7k}{}}
\newlabel{eq:cbw-HFGTprog:comp:InitOC}{{S7l}{6}{Weighted Least Squares Error Hetero-functional Graph State Estimation}{equation.7l}{}}
\newlabel{eq:cbw-HFGTprog:comp:FiniOC}{{S7m}{7}{Weighted Least Squares Error Hetero-functional Graph State Estimation}{equation.7m}{}}
\newlabel{eq:cbw-QPcanonicalform:3OC}{{S7n}{7}{Weighted Least Squares Error Hetero-functional Graph State Estimation}{equation.7n}{}}
\newlabel{eq:cbw-wlsehfgse-deviceModels}{{S7o}{7}{Weighted Least Squares Error Hetero-functional Graph State Estimation}{equation.7o}{}}
\@writefile{toc}{\contentsline {subsection}{\numberline {S2.1}Objective Function}{7}{subsection.2.1}\protected@file@percent }
\@writefile{toc}{\contentsline {subsection}{\numberline {S2.2}Equality Constraints}{7}{subsection.2.2}\protected@file@percent }
\citation{Thompson:2023:ISC-J51,Thompson:2024:ISC-J53,Thompson:2025:ISC-JR11,Farid:2022:ISC-AP80}
\citation{Thompson:2021:SPG-J44,Thompson:2020:SPG-C68}
\citation{Schoonenberg:2017:ISC-C60,Schoonenberg:2018:ISC-AP35,Schoonenberg:2019:ISC-BK04}
\citation{Khayal:2017:ISC-J35,Khayal:2021:ISC-J46}
\citation{Kelepouris:2006:IEM-C04,Schoonenberg:2017:IEM-J34}
\citation{Thompson:2025:ISC-JR11}
\citation{harris:2025:00}
\@writefile{toc}{\contentsline {subsection}{\numberline {S2.3}Inequality Constraints}{8}{subsection.2.3}\protected@file@percent }
\@writefile{toc}{\contentsline {subsection}{\numberline {S2.4}Device Model Constraints}{8}{subsection.2.4}\protected@file@percent }
\@writefile{toc}{\contentsline {section}{\numberline {S3}Sector Shares of Applied Nutrients}{9}{section.3}\protected@file@percent }
\newlabel{sec:cbw-SI-sector}{{S3}{9}{Sector Shares of Applied Nutrients}{section.3}{}}
\@writefile{lof}{\contentsline {figure}{\numberline {S3}{\ignorespaces Relative contribution of the agricultural and developed sectors to applied nitrogen and phosphorus on each land segment, 2024 Progress scenario (CAST input data).}}{9}{figure.caption.3}\protected@file@percent }
\newlabel{fig:cbw-map-sectorShar}{{S3}{9}{Relative contribution of the agricultural and developed sectors to applied nitrogen and phosphorus on each land segment, 2024 Progress scenario (CAST input data)}{figure.caption.3}{}}
\@writefile{toc}{\contentsline {section}{\numberline {S4}Land-Segment Edge-of-Stream and Edge-of-River Loads}{9}{section.4}\protected@file@percent }
\newlabel{sec:cbw-SI-lrs-eos}{{S4}{9}{Land-Segment Edge-of-Stream and Edge-of-River Loads}{section.4}{}}
\newlabel{LastPage}{{S2.4}{10}{Device Model Constraints}{page.10}{}}
\gdef\lastpage@lastpage{10}
\gdef\lastpage@lastpageHy{10}
\gdef \@abspage@last{10}
